# Supplementary material for: SNPL: Simultaneous Policy Learning and Evaluation for Safe Multi-Objective Policy Improvement
Source: arXiv:2503.12760 source file (2025-03-21)
Supplement: Supplementary file 1 [file additional_appendix.tex]

%\section{Additional Empirical Results}
%In this section, we provide (1) an ablation study to show the benefits of multiple testing, and (2) the effect of the regression baselines $\hat{\mu}_1, \hat{\mu}_0$ in improving detection power and expected improvement. 


%\subsection{Set-up for Additional Results}

%We add two modifications to our results shown in Section \ref{sec:empirics}: (1) two additional approaches to cutoff selection, which serve as an ablation study for CSPI-MT, and (2) two additional settings for our synthetic DGPs that illustrate when/why our approach improves over the HCPI $t$-test approach. For all results, we exclude the finite-sample version of HCPI due to similarly poor performance across all simulated settings. 

%\subsubsection{Additional Methods for Ablation Study}

%To provide an ablation study, we include two additional approaches to cutoff selection: (1) CSPI-P, which tests the cutoff with the highest estimated probability of passing, and (2) CSPI-MT(P), which initializes our multiple testing heuristic with the highest estimated improvement point. We provide the exact modifications below:
%\begin{itemize}
%    \item \textbf{CSPI-P}: In Algorithm \ref{alg:single_selection}, replace line 4 with 
%    $$c_1^* = \argmax_{c_i \in \Ccal} \widehat{P}(c_i, c_0), $$
%    and run Algorithm \ref{alg:MDR-HCPI} with $\omega = 0$.  
%    \item \textbf{CSPI-MT2}: In Algorithm \ref{alg:multi_selection}, replace line 4 with:
%    $$c_1^* = \argmax_{c \in \Ccal} \widehat{P}(c, c_0) \times \hat{\tau}(c),$$
%    and run Algorithm \ref{alg:MDR-HCPI} with $\omega = 1$. 
%\end{itemize}

%Comparing CSPI-MT with CSPI-P demonstrates the value of multiple testing, as opposed to simply testing just the first initialized cutoff. Comparing CSPI-MT with CSPI-MT2 justifies our choice of initializing the first cutoff as the cutoff with the highest estimated probability of passing, as opposed to the point with the highest expected improvement. We demonstrate that CSPI-MT maintains the high passing rates of testing just the single cutoff with the largest estimated passing probability, while increasing the expected improvement due to testing additional cutoff policies with larger estimated policy gains. 


%\subsubsection{Modulating Estimator Variance.}

%In addition to conducting our ablation study, we also provide an illustrative example of when and why CSPI and CSPI-MT outperform the asymptotic $t$-test approach in HCPI. The importance-weighted $t$-test approach used in HCPI differs from our efficient estimator defined in Section \ref{defn:policy_diff_est} by an propensity-weighted regression adjustment term involving $\hat{\mu}$. We modulate how much of $Y$'s variance is captured by the baseline regressor, $\hat{\mu}$ with the following modifications to our DGPs:
%$$X_1,X_2 \sim N(0, 16)\ , \quad \epsilon \sim N(0, 100)\ , $$
%while keeping all other settings the same as the simulation settings in Section \ref{sec:empirics}. 
%In this modified setting, our baseline regressor $\hat\mu$ captures less of the total variability of outcomes $Y$ relative to the unexplained variance $\epsilon$. This setting corresponds to scenarios where the estimator $\hat\mu$ only moderately reduces the lower confidence bound used for testing relative to that of the importance-weighted $t$-test approach of HCPI \cite{pmlr-v37-thomas15}.

%\subsection{Discussion of Results}

%\brian{running these simulations now...}



%\section{Additional Empirical Results for JOBS Semi-Synthetic Dataset.}




%\begin{proof}
    
%\end{proof}

%\begin{theorem}[]
    
%\end{theorem}


%\section{Datasets} \label{sec:appendix_datasets}
%\subsection{Visualization of Datasets}



%\begin{figure*}[htp]
  %\centering  \subfigure[caption 1]{\includegraphics[scale=0.2]{figures/EI_200sims_samples_400_1600_gamma_01.png}}\quad
  %\subfigure[caption 2]{\includegraphics[scale=0.2]{figures/PR_200sims_samples_400_1600_gamma_01.png}}
%\end{figure*}




%\subsection{Visualization of Jobs Dataset} \label{subsec:appendix_behagel}


%\section{Extended Empirical Details} \label{sec:appendix_empirical_results}

%\subsection{Modifications to HCPI for Policy Differences }
